# Supplementary material for: Physics-Aware Neural Implicit Solvers for multiscale, parametric PDEs with applications in heterogeneous media
Source: arXiv:2405.19019 source file (2024-05-29)
Supplement: Supplementary file 1 [file appendixHcalc.tex]

\newpage
\section{Loss and Gradient Estimation of $H(\bphi)$}
\label{appendix:HEstimation}
As mentioned in section \ref{sec:GreedyAlgorithm} the loss function for finding the next best virtual observable to add is equal to $H(\bphi)=KL\left(q_{n, \bpsi}(\bx, \by) || p_{n+1}(\bx, \by)\right)$. For reasons that will become apparent next we consider $H(\bphi) = KL\left(q_{n, \bpsi}(\bx, \by) || p_{n+1}(\bx, \by)\right) - KL\left(q_{n, \bpsi}(\bx, \by)||p_{n}(\bx, \by)\right)$ for calculating the gradients of $H$, which will yield the same result since the second term is independent of the weighting functions $w_{n+1}(\bs{s})$. Thus we can write

\be
\begin{array}{ll}
KL\left(q_{n, \bpsi}(\bx, \by) || p_{n+1}(\bx, \by)\right) - KL\left(q_{n, \bpsi}(\bx, \by)||p_{n}(\bx, \by)\right) & = - \left< \log \frac{ p(\hat{r}_{n+1} | \bx, \by) p(\hat{\bs{R}}_n | \bx, \by) p(\bx, \by) }{ p(\hat{\bs{R}}_n\cup \hat{r}_{n+1})~q_n(\bx, \by)} \right>_{q_n} +\left< \log \frac{ p(\hat{\bs{R}}_n | \bx, \by) p(\bx, \by) }{ p(\hat{\bs{R}}_n)~q_n(\bx, \by)}  \right>_{q_n}\\
 & =-\left< \log p(\hat{r}_{n+1} | \bx, \by)\right>_{q_n}+\log \frac{ p(\hat{\bs{R}}_n\cup \hat{r}_{n+1}) }{ p(\hat{\bs{R}}_n) }
 \label{eq:dkl}
\end{array}
\ee

The first term can be readily approximated and is proportional to the square residual associated  with $w_{n+1}$ averaged over $q_{n, \bpsi}(\bx, \by)$. Hence it promotes test functions which according to our current state of knowledge, produce the highest residuals.
The second term is a bit more subtle and assesses the ratio of normalizing constants. The latter can be thought of as the hypervolume in the $\bx, \by-space$ of all such points that have non-zero posterior.  Only the numerator depends on $w_{n+1}(\bs{s})$ and maximizing provides a regularization over the effect of the new residual.

The term $p(\hat{\bs{R}}_n)$, can be ignored since it is independent of $\bphi$ and constant for each individual optimization procedure for acquiring a new test function $w_{n+1}(\bs{s})$. Hence, we propose approximating just the numerator as: 
\be
\begin{array}{ll}
 \log p(\hat{\bs{R}}_n\cup \hat{r}_{n+1}) & = \log \int  \pi_{n+1}(\bx, \by) ~d\bx d\by \\
  & = \log  \left<  \frac{\pi_{n+1}(\bx, \by) }{q_{n, \bpsi}(\bx, \by)} \right>_{q_{n, \bpsi}(\bx, \by)} \\
  & \approx \log \frac{1}{N_z} \sum_{i=1}^{N_z} \frac{ p(\hat{r}_{n+1} | \bx^{(i)}, \by^{(i)}) p(\hat{\bs{R}}_n | \bx^{(i)}, \by^{(i)}) p(\bx^{(i)}, \by^{(i)}) }{q_n(\bx^{(i)}, \by^{(i)})}
 \end{array}
\ee
Assuming $q_{n+1, \bpsi}(\bx, \by)$ is parametrized by $\bp$ and if $H(\bp)= KL\left(q_{n, \bpsi}(\bx, \by) || p_{n+1}(\bx, \by)\right) - KL\left(q_{n, \bpsi}(\bx, \by)||p_{n}(\bx, \by)\right)$, we obtain:
\be
\begin{array}{ll}
 H(\bp) & = -\left< \log p(\hat{r}_{n+1} | \bx, \by\right>_{q_n} + \log p(\hat{\bs{R}}_n\cup \hat{r}_{n+1})  \\
 & \approx - \frac{1}{N_z} \sum_{i=1}^{N_z} \log p(\hat{r}_{n+1} | \bx^{(i)}, \by^{(i)})+\log \frac{1}{N_z} \sum_{i=1}^{N_z} \frac{ p(\hat{r}_{n+1} | \bx^{(i)}, \by^{(i)}) p(\hat{\bs{R}}_n | \bx^{(i)}, \by^{(i)}) p(\bx^{(i)}, \by^{(i)}) }{q_{n,\bpsi}(\bx^{(i)}, \by^{(i)})} \\
 & = - \frac{1}{N_z} \sum_{i=1}^{N_z} \log p(\hat{r}_{n+1} | \bx^{(i)}, \by^{(i)})+\log \frac{1}{N_z} \sum_{i=1}^{N_z} \frac{ p(\hat{r}_{n+1} | \bx^{(i)}, \by^{(i)}) \pi_n( \bx^{(i)}, \by^{(i)})  }{q_{n,\bpsi}(\bx^{(i)}, \by^{(i)})}
\end{array}
\ee
which upon differentiation leads to:
\be
\frac{\pa H}{\pa \bp}= \lambda \left( \sum_{i=1}^{N_z} (\frac{1}{N_z}  -v_i)~ r_{\bp}(\bx^{(i)}, \by^{(i)}) \frac{\pa r_{\bp}(\bx^{(i)}, \by^{(i)})}{\pa \bp}  \right)
\ee
where $v_i=\cfrac{ e^{-\frac{\lambda}{2} r_{\bp}^2(\bx^{(i)}, \by^{(i)}) }  \pi_n(\bx^{(i)}, \by^{(i)}) /q_{n,\bpsi}(\bx^{(i)}, \by^{(i)}) }{ \sum_{j=1}^{N_z} e^{-\frac{\lambda}{2} r_{\bp}^2(\bx^{(i)}, \by^{(j)}) }\pi_n(\bx^{(i)}, \by^{(j)}) /q_{n,\bpsi}(\bx^{(i)}, \by^{(j)}) }$ and $\frac{\pa r_{\bp}(\bx^{(i)}, \by^{(i)})}{\pa \bp}$ is calculated using automatic differentiation.
